# Supplementary material for: Connecting Distributed Pockets of EnergyFlexibility through Federated Computations:Limitations and Possibilities
Source: arXiv:2009.10182 source file (2020-09-21)
Supplement: Supplementary file 1 [file appendix.tex]

This section presents a mathematical justification that any limit point of the proposed algorithm in \eqref{intradense} is optimal solution of the underlying optimization problem in \eqref{generalproblem}. Moreover, it presents a sufficient condition for convergence of the proposed federated updates.

\indent It can shown that a fixed point of the proposed iterative federated scheme  satisfies the optimality conditions of the original optimization problem \eqref{generalproblem}. The author in \cite{Mohammadi2016} has proved that any fixed point of the proposed updates \eqref{y_update} satisfies all of the first order optimality conditions of the original problem presented by \eqref{generalproblem}.

Moreover, it can be proven that if the underlying optimization problem formulation \eqref{generalproblem} is convex and has a feasible solution that lies in the feasible space defined by the corresponding constraint set and if the federated updates \eqref{y_update} converges to a fixed point, then that fixed point is the optimal solution of the original optimization problem. 

Note that in \eqref{y_update} tuning parameters have a considerable impact on convergence speed of the federated computations. Typical conditions that ensure convergence \cite{kar2012distributed} include:
\begin{enumerate}
    \item Sufficient regularity of the local functions 
    \item Connectivity of the inter-agent communication graph.
    \item The following conditions on the $\alpha^c$ and $\alpha^I$ parameters:
    \begin{itemize}
        \item $\alpha^c(k) \geq 0$ and $\alpha^I(k) \geq 0$ \vspace{1mm}
        \item As $k \rightarrow \infty$, $\alpha^c(k) \rightarrow 0$ and $\alpha^I(k) \rightarrow 0$\vspace{1mm}
        \item $\sum \alpha^I(k)=\sum \alpha^C(k)=\infty$\vspace{1mm}
        \item As $k \rightarrow \infty$, $\alpha^C(k)/\alpha^I(k)\rightarrow \infty$
    \end{itemize}
\end{enumerate}
